# Supplementary material for: Non-convex Bayesian Learning via Stochastic Gradient Markov Chain Monte Carlo
Source: arXiv:2305.19350 source file (2023-05-30)
Supplement: Supplementary file 1 [file ap-about-appendices.tex]

\ProvidesFile{ap-about-appendices.tex}[2021-08-23 about the appendicies appendix]

\begin{VerbatimOut}{z.out}
\chapter{ABOUT THE APPENDICES}

% Use single spacing in the appendices from now on to save space.
\ZZbaselinestretch{1}

\textcolor{red}{%
  \textbf{%
    These appendices are single-spaced to save space.
    Your thesis should use the default~1.5 line spacing.%
  }%
}

There are two groups of appendices.
The first group are general appendices;
the second group are domain-specific appendices.

These appendices are a series of examples.
They are a work in progress.

Each example consists of some \LaTeX\ output
followed by the corresponding input lines.
Some \LaTeX\ input lines only define things
and don't produce any output.
Each chunk in the input file begins with
\verb+\begin{VerbatimOut}{z.out}+
then has the \LaTeX\ input for the example,
% Don't literally end VerbatimOut on next line.
and ends with {\tt \char'134 end\char'173 VerbatimOut\char'175},
followed by a blank line,
followed by a line that begins with
\verb+\My+.

\end{VerbatimOut}

\MyIO

\begin{VerbatimOut}{z.out}

\section{Paragraphs}

This is the first paragraph.
Paragraphs are separated by blank lines.

This is the second paragraph.

\section{Section Heading}

This is a sentence.
This is a sentence.
This is a sentence.
This is a sentence.
This is a sentence.

\subsection{Subsection heading}

This is a sentence.
This is a sentence.
This is a sentence.
This is a sentence.
This is a sentence.

\subsubsection{Subsubsection heading}

This is a sentence.
This is a sentence.
This is a sentence.
This is a sentence.
This is a sentence.
\end{VerbatimOut}

\MyIO

\begin{VerbatimOut}{z.out}

\section{Text math}

If items in a list are narrow like these Greek characters,\\
    \I2 \verb+$\alpha$, $\beta$, and $\gamma$+\\
I'd input the line like this\\
    \I2 \verb+$\alpha$,~$\beta$, and~$\gamma$+\\
where the \verb+~+ is a tie
that ties together what's before and after it on the same line of the output
\cite[page~92]{knuth2012}.

This text is the correct length to show what happens with and without ties:
$\alpha$,
$\beta$,
and $\gamma$.
See how the line gets split
and the~$\gamma$ is at the beginning of the line?

This text is the correct length to show what happens with and without ties:
$\alpha$,~$\beta$,
and~$\gamma$.
See how the line gets compressed a little bit so the~$\gamma$
is not at the beginning of the line?
\end{VerbatimOut}

\MyIO
