# Supplementary material for: Non-convex Bayesian Learning via Stochastic Gradient Markov Chain Monte Carlo
Source: arXiv:2305.19350 source file (2023-05-30)
Supplement: Supplementary file 2 [file ap-chapter-appendices.tex]

\ProvidesFile{ap-chapter-appendices.tex}[2021-08-23 chapter appendices appendix]

\begin{VerbatimOut}{z.out}
\chapter{CHAPTER APPENDICES}

Using \verb+\chapterappendix+ or \verb+\chapterappendices+
in the first chapter will number sections, for example,
1.1, 1.2, 1.A.

Using \verb+\chapterappendix+ or \verb+\chapterappendices+
in the first appendix will number sections, for example,
A.1, A.2, A.A.

Only use \verb+\chapterappendix+ or \verb+\chapterappendices+
in chapters.
Using them in appendices is too confusing.

\section{This is a section headings}

This is a paragraph.

Use \verb+\chapterappendix+ or \verb+chapterappendices+
to make sections until the end of the next chapter
be appendices.

\chapterappendix

\section{This is a chapter appendix}

This is a paragraph.
\end{VerbatimOut}

\MyIO
